# Supplementary material for: Statistics of overtakes by a tagged agent
Source: arXiv:1804.07280 source file (2018-04-19)
Supplement: Supplementary file 1 [file supplmental.pdf]

# Statistics of overtakes by a tagged agent: Supplemental material

Santanu Das,[1] Deepak Dhar,[2] and Sanjib Sabhapandit[1]

[1]*Raman Research Institute, Bangalore 560080, India*

[2]*Indian Institute of Science Education and Research (IISER), Pune 411008, India*

(Dated: April 17, 2018)

In the main text, we have considered a one-dimensional infinite lattice where at each site there sits an agent carrying a velocity, which is drawn initially for each agent independently from a common distribution $\rho(v)$. The system evolves by a Markovian dynamics where a pair of agents at adjacent sites $i$ and $i+1$ exchange their positions with the rate $r = \theta(v_i - v_{i+1})(v_i - v_{i+1})^\alpha$ where $v_i$ is the velocity at site $i$ before the exchange. The agents retain their respective velocities with them at all times, and hence, the velocity $v_i$ at a given site $i$ keeps changing with time. We have studied the statistics of the net displacement of a tagged agent $m(t)$ on the lattice, in a given duration $t$, for two different cases: $\alpha = 0$ and $\alpha = 1$. Here we provide additional materials to support the main text.

1. For the $\alpha = 0$ case, we have mentioned in the main text that the variance of the displacement of a tagged agent crosses over from the initial $\langle m^2 \rangle_c \propto t$ behavior to the long time behavior $\langle m^2 \rangle_c \propto t^{4/3}$, where the crossover time depends on the velocity $v_0$ of the tagged agent. Here we illustrate this in Fig. 1.

2. In Fig. 2 of the main text, we have illustrated that the conditional probability density function (PDF) $p_2(c, t|\bar{c})$ for $\bar{c} \to \pm 1$, is given by the Gaussian distribution, coming from the random walk description of the process, while at the central part $p_2(c, t|\bar{c})$ is described by Eq. (4) of the main text. Here instead, we look at the conditional PDF $p_1(c, t|v_0)$ itself at fix times for different values of $v_0$. If $v_0$ is such that the characteristic time $t_*(v_0)$ is large compared to our observation times, the dynamics of the tagged agent can be described by random walk as shown by the two figures on the first row of Fig. 2. The Gaussian distribution describes the typical fluctuation for the displacement of a random walk only at the scale of $\sqrt{t}$ about the mean [see the first figure on the first row of Fig. 2]— unless the jump distribution itself is Gaussian, where fluctuations of the displacement at all scales are also Gaussian. To confirm that the jump process at $t \ll t_*(v_0)$ is indeed well-described by the random walk, we also look at the large fluctuations at the scale of $t$, which are described by the large deviation form discussed in Sec. I below. The second figure on the first row of Fig. 2 indeed affirms this. In Fig. 2 of the main text, we have shown that for small $\bar{c}$, the conditional PDF $p_2(c, t|\bar{c})$, when shifted and scaled appropriately, is given by the scaling function $G_{\text{scaling}}(y)$, that is discussed in the main text. Here, in the figure on second row of Fig. 2, we illustrate that if $v_0$ is such that $t_*(v_0)$ is small compared to our observation times, the conditional PDF $p_1(c, t|v_0)$, when shifted and scaled appropriately, is given by the scaling function $G_{\text{scaling}}(y)$.

3. In Fig. 3 (a), (b), (c), and (d) of the main text, we have plotted the simulation results for the PDF of $c = m(t)/t$ for four choices of the velocity distributions (the exact form of the distributions are given in Sec. II below) and compared them with Eq. (5). We find very good agreement at large times. Note that Eq. (5) of the main text has been obtained by using a Gaussian distribution for $p_2(c, t|\bar{c})$. As mentioned above, and illustrated in Fig. 2, the large fluctuation are better described by the large deviation form of the PDF, which also include the typical fluctuations. Therefore, here we use the large deviation form Eq. (S8) in Eq. (3) of the main text to numerically obtain the PDF $p(c, t)$ and compare this with simulation results in Figure 3, which gives better agreement than Eq. (5) of the main text. This confirms that, the tails of $(p(c, t)$ indeed comes from the random walk description.

4. For the $\alpha = 1$ case, we have mentioned in the main text that the variance of the displacement of a tagged agent crosses over from the initial $\langle m^2 \rangle_c \propto t$ behavior to the long time marginally superdiffusive behavior. Here we illustrate this in Fig. 4.

5. In Fig. 5 we illustrate that at early times $t \ll t_\#(v_0)$, for the $\alpha = 1$ case also, the jump process of a tagged agent is described by the random walk. We do this by showing that the conditional PDF of the appropriately shifted and scaled displacement $y = (m - \bar{c}t)/\sqrt{t}$, for $t \ll t_\#(v_0)$ is Gaussian. We also look at the large fluctuations and find that it is given by the large deviation form Eq. (S9) for the random walk with the appropriate hopping rates. For $t \gg t_\#(v_0)$, the conditional PDF of the appropriately scaled displacement is again Gaussian — however, with a scaling marginally different from $\sqrt{t}$.

6. The exact anomalous scaling for the scaled displacement for $t \gg t_\#(v_0)$, for the $\alpha = 1$ case, is difficult to determine based on our numerics, as shown in Fig. 6.

7. In Fig. 7 we give additional support that the tails of $p(c,t)$ for $\alpha = 1$ case also comes from the random walk description of the jump process for an tagged agent. Here we magnify the tails part of the plots in Fig. (4) of the main text, and show that if we use the large deviation form for $p_1(c,t|v_0)$ to compute $p(c,t)$ in Eq. (2) of the main text, the simulation results for the tails agree even at smaller times.

## I. LARGE DEVIATION FUNCTION OF FOR THE PDF OF THE DISPLACEMENT OF A RANDOM WALK ON A ONE-DIMENSIONAL LATTICE, EVOLVING IN CONTINUOUS TIME

Consider a random walk on a one-dimensional infinite lattice evolving as a continuous time Markov process. The random walker on the lattice jumps to right and left adjacent sites with homogeneous and time independent rates $p_r$ and $p_l$ respectively. The time evolution of the probability distribution $P(m,t)$ of the walker of being at the site $m$ at time $t$ is given by the master equation

$$\frac{d}{dt}P(m,t) = p_r\ P(m-1,t) + p_l\ P(m+1,t) - (p_r + p_l)\ P(m,t). \tag{S1}$$

We consider initial condition $P(m,0) = \delta_{m,0}$. The characteristic function is given by

$$\tilde{P}(k,t) \equiv \langle e^{ikm} \rangle = e^{\lambda(k)t} \tag{S2}$$

where the cumulant generating function (CGF) is given by

$$\lambda(k) = p_r\left(e^{ik} - 1\right) + p_l\left(e^{-ik} - 1\right). \tag{S3}$$

Evidently, the $n$-th cumulant is

$$\langle m^n(t) \rangle_c = [p_r +\ (-1)^n p_l]\ t. \tag{S4}$$

The distribution at large time can be obtained by inverting the characteristic function using saddle-point approximation, which for the scaled variable $c = m/t$ yields

$$P(c,t) \simeq \sqrt{\frac{t}{2\pi}}\ \frac{e^{-t\ \phi(c)}}{\sqrt{\phi''(c)}} \tag{S5}$$

with large deviation function (LDF) [1]

$$\phi(c) = c\ \text{Log}\left[\frac{c + \sqrt{c^2 + 4p_r p_l}}{2p_r}\right] + (p_r + p_l) - \sqrt{c^2 + 4p_r p_l} \tag{S6}$$

and $\phi''(c) = \sqrt{c^2 + 4p_r p_l}$. By expanding around its average $\bar{c}$, one can also recover the well known Gaussian approximated result (GUS)

$$P(c,t) = \frac{1}{\sqrt{2\pi\sigma_t^2}}\ e^{-\frac{(c-\bar{c})^2}{2\ \sigma_t^2}} \tag{S7}$$

where $\bar{c} = \langle m(t) \rangle_c / t = p_r - p_l$ and its variance $\sigma_t^2 = \langle m^2(t) \rangle_c / t^2 = (p_r + q_l)/t$.

### A. Case I : ($\alpha = 0$)

In this case, in the main text we have used the rates $p_r(v_0) \equiv \rho_+(v_0)$ and $p_l(v_0) \equiv \rho_-(v_0)$ for a tagged particle of velocity $v_0$. By using these relations we have plotted the distribution associated with LDF and GUS in the first row of Fig. 2. Now, using the PDF of the form of Eq. (S5) with the fact $p_r(v_0) + p_l(v_0) = 1$, the conditional PDF $p_2(c,t|\bar{c})$ in the main text can be written as:

$$p_2(c,t|\bar{c}) = \sqrt{\frac{t}{2\pi}}\ \frac{e^{-t\ \phi(c,\bar{c})}}{\sqrt{\phi''(c,\bar{c})}} \tag{S8}$$

with $\phi(c,\bar{c}) = c\ \text{Log}\left[\frac{c+\sqrt{c^2+1-\bar{c}^2}}{1+\bar{c}}\right] + 1 - \sqrt{c^2 + 1 - \bar{c}^2}$ and $\phi''(c,\bar{c}) = \sqrt{c^2 + 1 - \bar{c}^2}$. Using this result in Eq.(3) in main text we numerically computed the exact tail behavior of the scaled net overtaking distribution $p(c,t)$ as shown in Fig. 3.

### B. Case II : ($\alpha = 1$)

In this case, in the main text we have used $p_r(v_0) \equiv \rho_R(v_0)$ and $p_l(v_0) \equiv \rho_L(v_0)$ for a tagged particle of velocity $v_0$. By using these relations we have plotted the distribution associated with LDF and GUS in the first row of Fig. 5. Now, using the PDF of the form of Eq. (S5) with the fact $p_r(v_0) + p_l(v_0) = \sigma^2(v_0)$, the conditional PDF $p_1(c,t|v_0)$ in the main text can be written as:

$$p_1(c,t|v_0) = \sqrt{\frac{t}{2\pi}}\,\frac{e^{-t\,\phi(c,v_0)}}{\sqrt{\phi''(c,v_0)}} \tag{S9}$$

with $\phi(c,v_0) = c\,\mathrm{Log}\left[\frac{c+\sqrt{c^2+\sigma^4(v_0)-\bar{c}^2(v_0)}}{\sigma^2(v_0)+\bar{c}(v_0)}\right] + \sigma^2(v_0) - \sqrt{c^2+\sigma^4(v_0)-\bar{c}^2(v_0)}$ and $\phi''(c,v_0) = \sqrt{c^2+\sigma^4(v_0)-\bar{c}^2(v_0)}$. Using this result alongside the explicit form velocity distribution $\rho(v_0)$ in Eq.(2) in main text we numerically computed the exact tail behavior of the scaled net overtaking distribution $p(c,t)$ as shown in Fig. 7.

## II. THE FOUR VELOCITY DISTRIBUTIONS USED IN THE MAIN TEXT:

In the main text we have shown numerical results for four different velocity distributions. The distribution are respectively

$$(i)\qquad \rho(v) = \frac{1}{2}\ ;\ v \in [-1:1] \qquad \text{(Uniform)}, \tag{S10}$$

$$(ii)\qquad \rho(v) = \frac{e^{-\frac{v^2}{2}}}{\sqrt{2\pi}}\ ;\ v \in [-\infty:\infty] \qquad \text{(Gaussian)}, \tag{S11}$$

$$(iii)\qquad \rho(v) = e^{-v}\ ;\ v \in [0:\infty] \qquad \text{(Exponential)}, \tag{S12}$$

$$(iv)\qquad \rho(v) = \frac{\nu}{v^{1+\nu}}\ ;\ v \in [1:\infty] \qquad \text{(Power law)}. \tag{S13}$$

The first two distributions are symmetric while the last two are asymmetric with respect to the mean of the distribution $\langle v \rangle$. From the other viewpoint, the first three distributions have all finite moments while the last one have diverging moments. The behavior of the power-law distribution is completely characterized by its exponent $\nu > 0$. In the main text, for power-law, all the results have shown for $\nu = 2.5$.

---

[1] H. Touchette, Phys. Rep. **478**, 1 (2009).

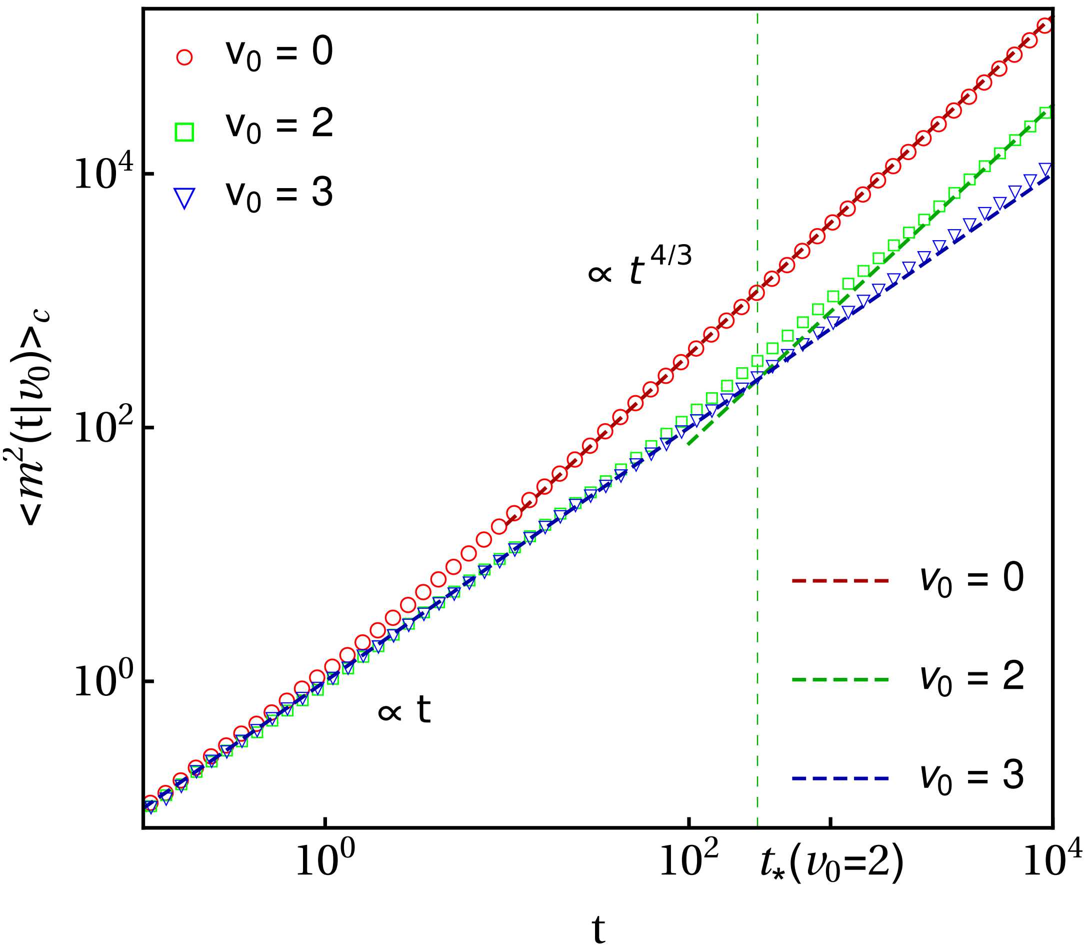


FIG. 1: Simulation results (shown by discrete points), illustrating the crossover from the initial $\propto t$ behavior to the long-time $\propto t^{4/3}$ behavior, for the variance of the displacement of the tagged particle for the $\alpha = 0$ case discussed in the main text. Three different values of the tagged velocity $v_0 = 0$, 2, and 3 are considered while the initial velocities of the other particles are drawn independently from a Gaussian distribution. The finite size effects do not show up till the final measurement time considered in the simulations, for a system of size $N = 2 \times 10^3$ with periodic boundary condition. For $v_0 = 0$ an anomalous growth $\propto t^{4/3}$ is clearly noticeable. The result for the intermediate velocity $v_0 = 2$ is showing a transition from the initial $\propto t$ behavior to the long-time $\propto t^{4/3}$ behavior. The third one $v_0 = 3$ mostly shows the linear growth $\propto t$, with a hint of the crossover towards the end. The dashed lines plot the analytical results which show a good agreement with the corresponding numerical results. The vertical dashed line is showing an approximate transition time $t_*(v_0)$ between the initial linear growth to the long-time non-linear one for velocity $v_0 = 2$.

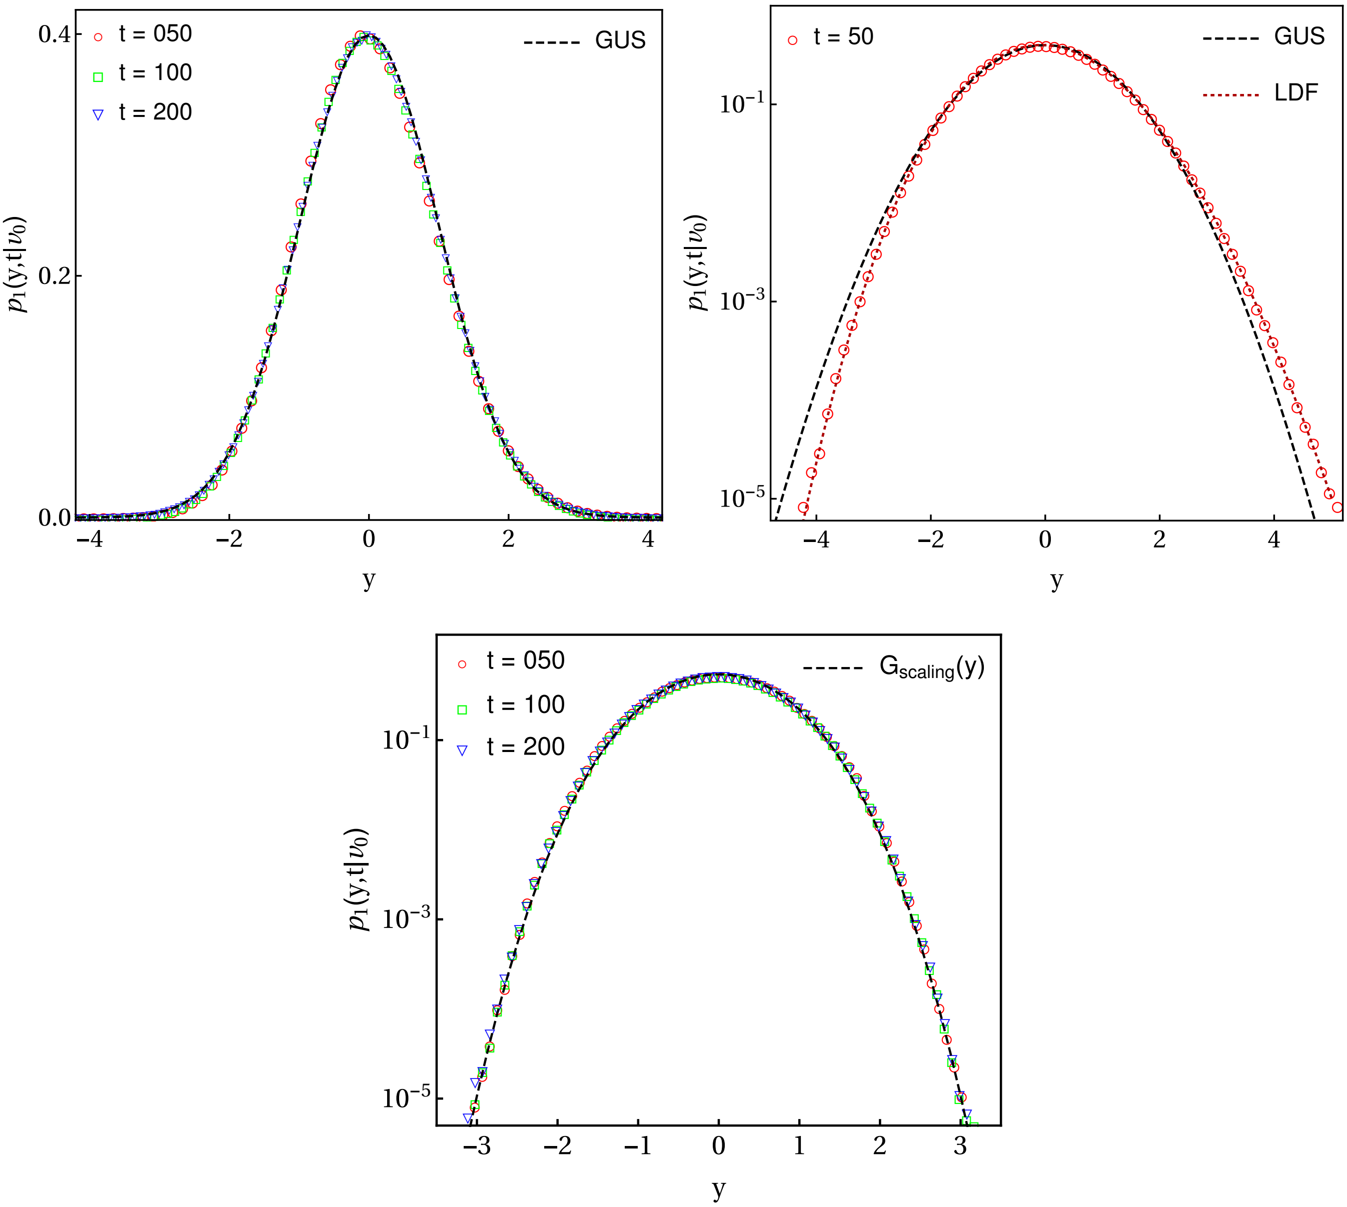


FIG. 2: Conditional PDF of the displacement $m(t)$ of the tagged particle with a given velocity $v_0$ in the two different limits (i) $t << t_*(v_0)$ (the two figures on the first row) and (ii) $t >> t_*(v_0)$ (the figure on the second row), for the $\alpha = 0$ case discussed in the main text. To satisfy those limits we have conveniently considered the tagged velocity $v_0 = 3$ for the two figures on the first row and $v_0 = 0$ for the figure on the second row. In the first figure on the first row, the simulation results, denoted by points, for the PDF of the scaled displacement $y \propto (m - \bar{c}t)/\sqrt{t}$, are plotted together with a Gaussian distribution denoted by the dashed line. In the second figure on the first row, we use log-linear scale to show that a large fluctuations deviates from the Gaussian (shown by the dashed line), which are better described by the large deviation result shown by the dotted line. The figure on the second row demonstrates that in the opposite limit $t >> t_*(v_0)$, with the appropriate scaling $y \propto t^{-2/3}(m - \bar{c}t)$, the PDFs for different times collapse onto the scaling function $G_{\text{scaling}}(y)$ (shown by dashed line) that is discussed in the main text.

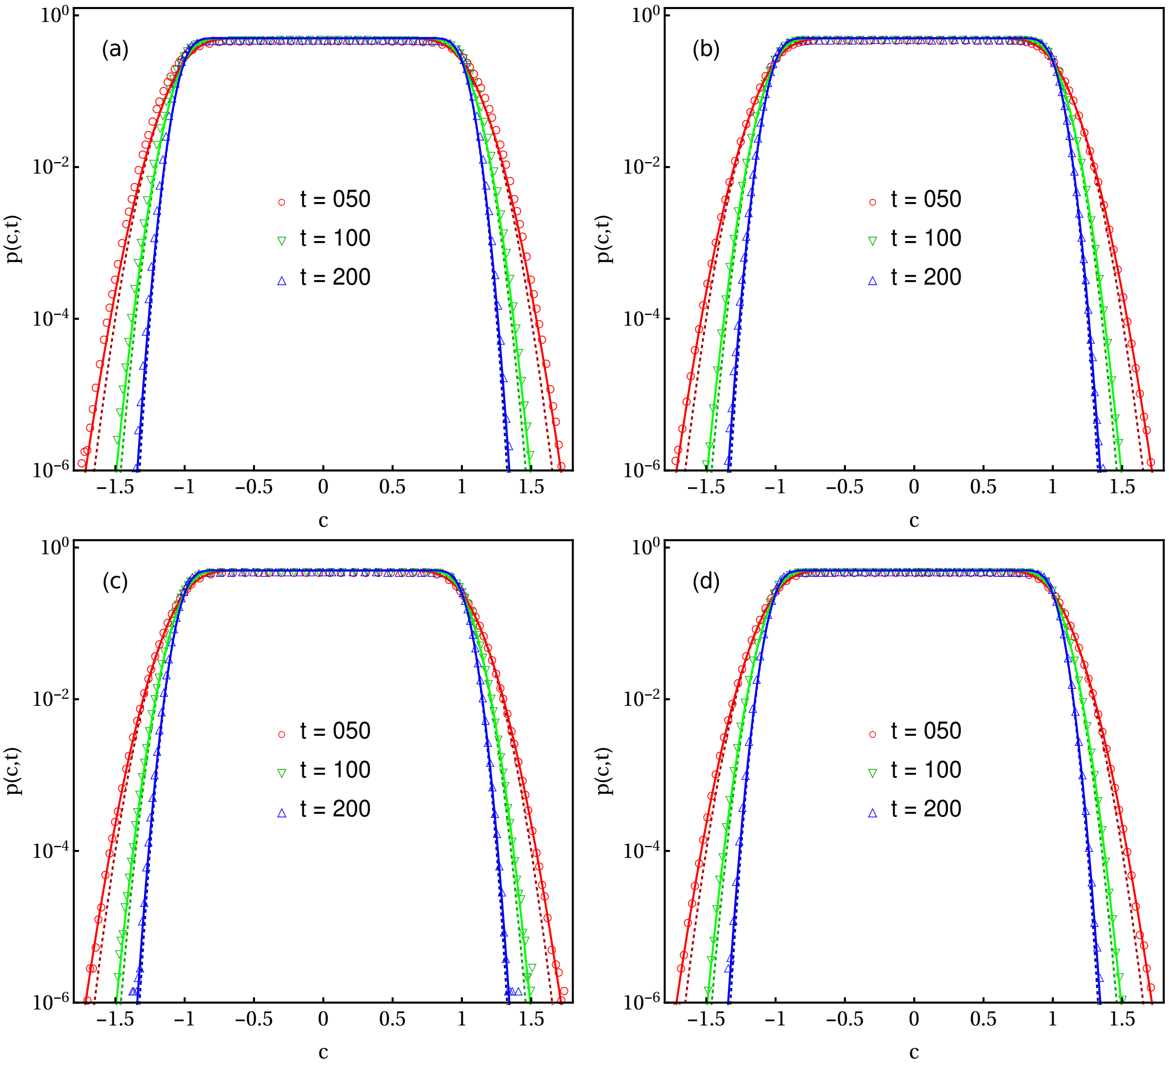


FIG. 3: Probability density function $p(c,t)$ of the scaled net overtakings $c = m(t)/t$ are plotted at three different times, for $\alpha = 0$ case discussed in the main text, with four different choices of the initial velocity distribution, namely, (a) uniform (b) Gaussian (c) exponential and (d) power-law distributions. The discrete points in each plot are the simulation results, which show very good agreements with the results coming from the analysis of the large deviation form of the conditional distribution $p_2(c,t|v_0)$ (as shown by the bold lines). The corresponding results coming from the Gaussian approximation, are plotted by the dashed lines, for which the agreements at the tails improve as $t$ becomes larger.

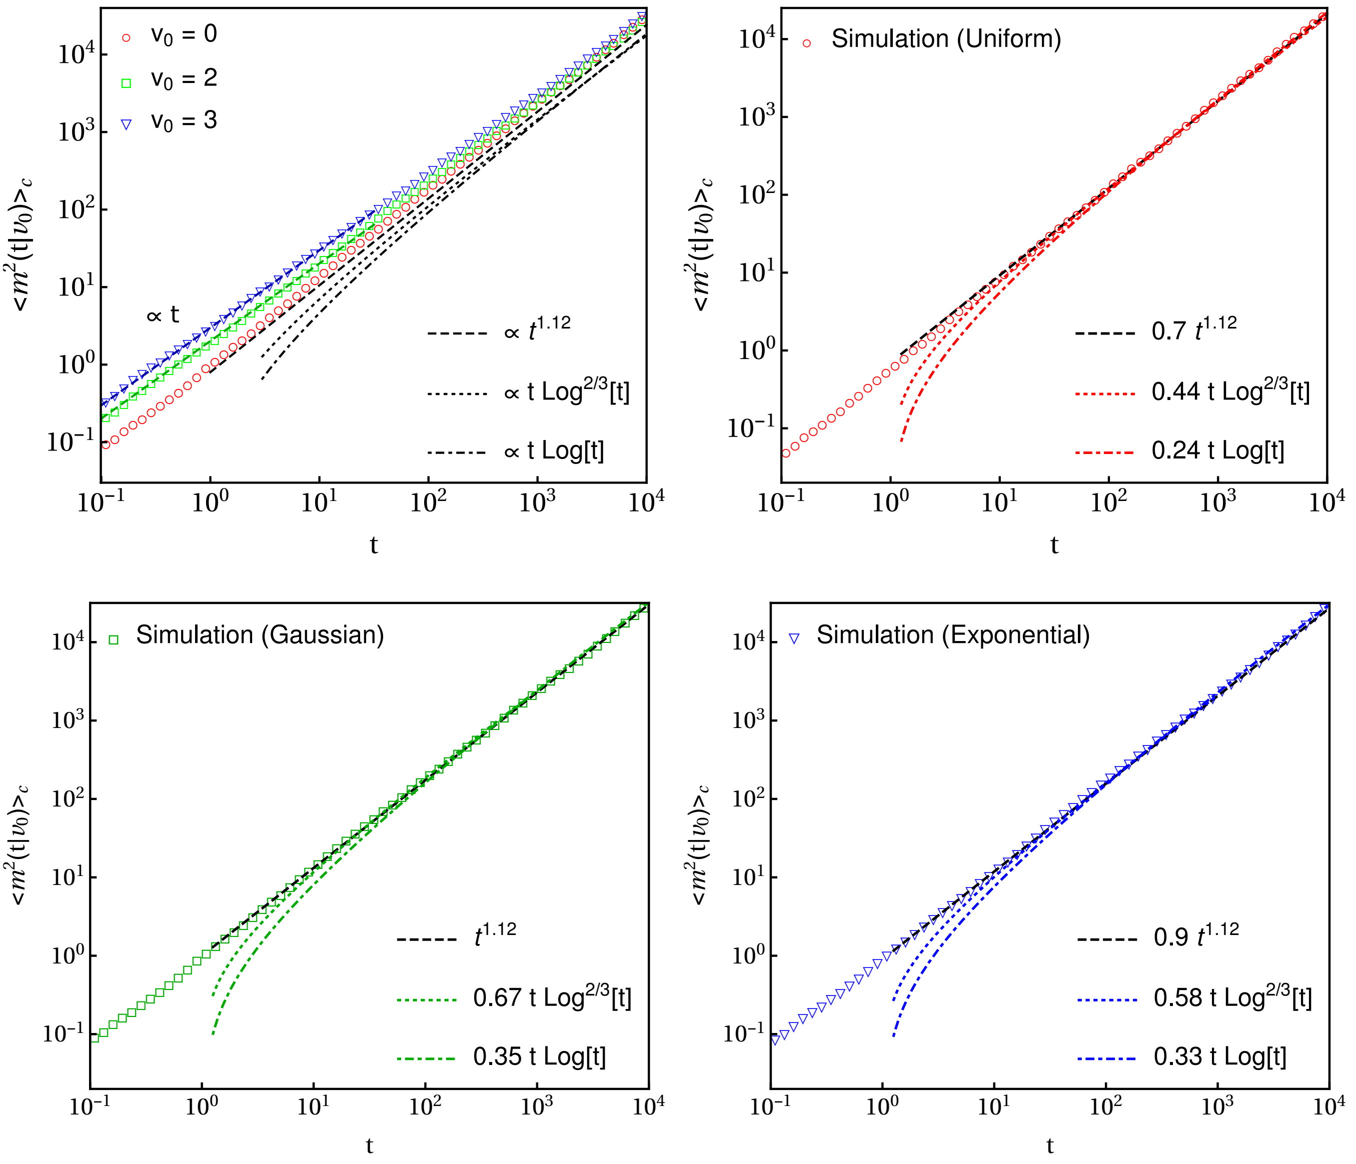


FIG. 4: Simulation results for the variance of the displacement of the tagged particle for the $\alpha = 1$ case discussed in the main text. In the first figure on first row, we plot the variance for three different values of the tagged velocity, while the velocities of the other particles are drawn independently from a symmetric Gaussian distribution. The finite size effects do not show up till the final measurement time considered in the simulations, for a system of size $N = 10^4$ with periodic boundary condition. The data for the largest tagged velocity $v_0 = 3$ shows only a linear growth $\propto t$ in time. The data for the intermediate value $v_0 = 2$ is showing a transition from the initial $\propto t$ behavior to an anomalous long-time behavior. For $v_0 = 0$ an anomalous growth is clearly noticeable. In the second figure on the first row and the first and second figures on the second row, we plot the variance of a tagged particle of velocity $v_0 = \langle v \rangle$ for uniform, Gaussian and exponential distributions respectively, highlighting the anomalous growth. The exact anomalous behavior is not clear as it matches with both $\propto t^{1.12}$ (as shown by bold lines) and $\propto t\,[\mathrm{Log}(t)]^{2\gamma}$. Our simulation results show good agreement for both $\gamma = 1/3$ (as shown by dotted lines) and $\gamma = 1/2$ (as shown by dotdashed lines).

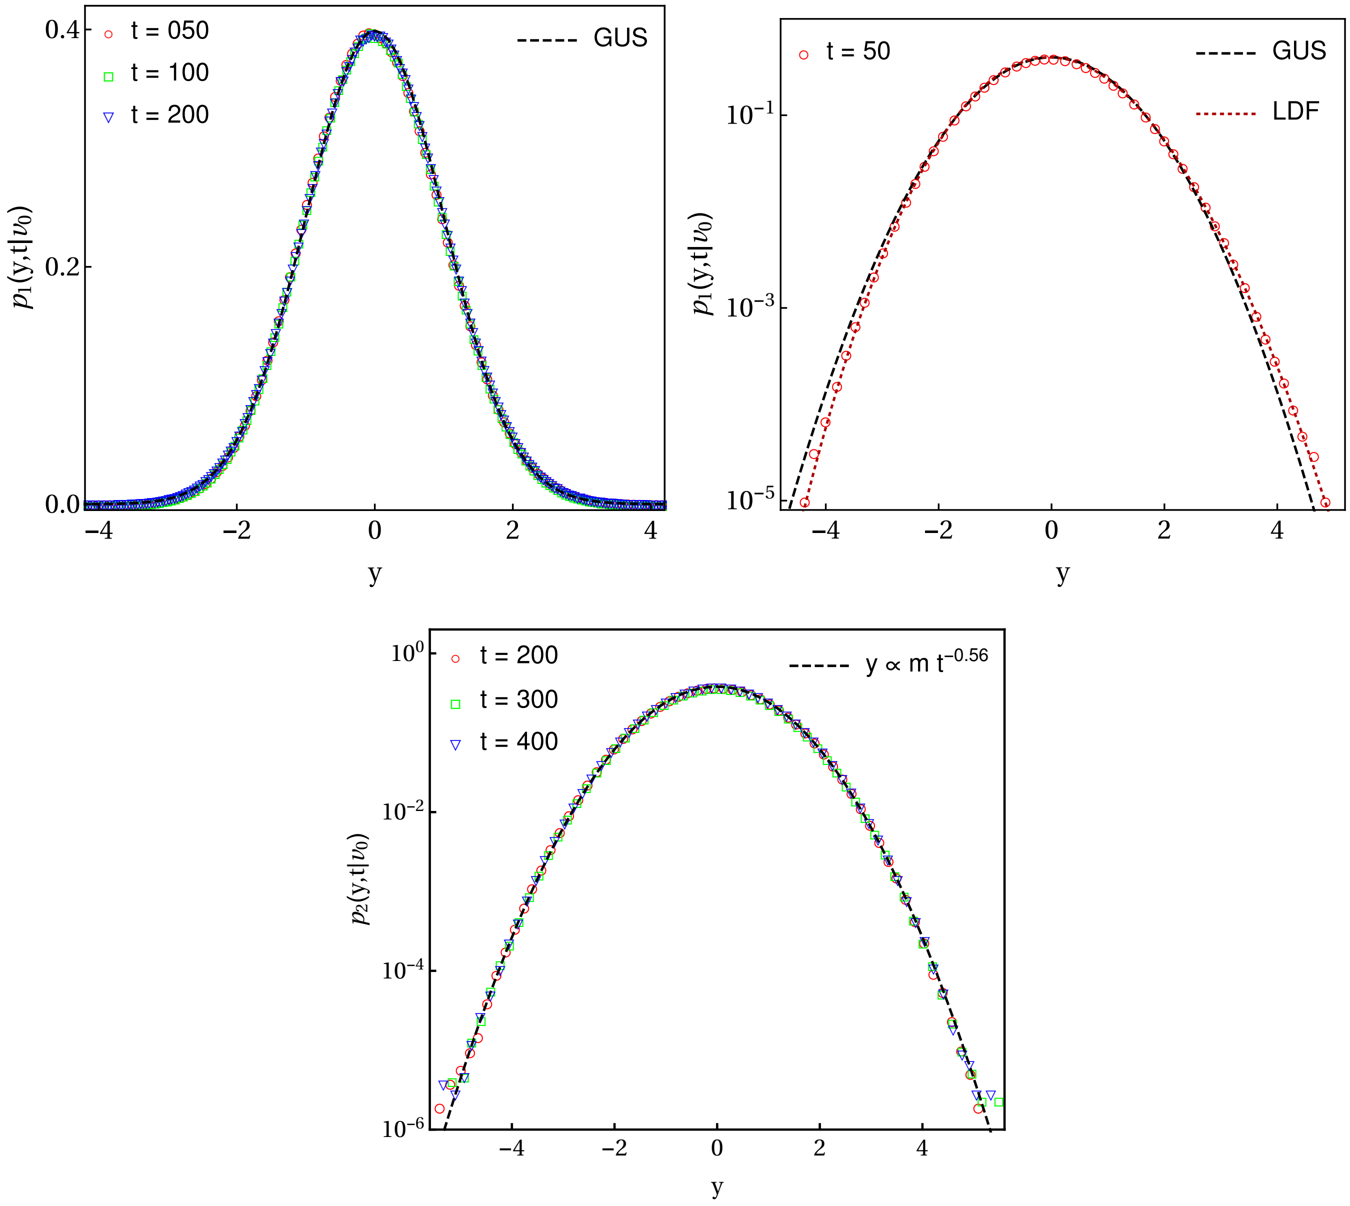


FIG. 5: Conditional PDF of the displacement of a tagged particle with a given velocity in the two different limits (i) $t << t_{\#}(v_0)$ (figures on the first row) and (ii) $t >> t_{\#}(v_0)$ (the figure on the second row), for the $\alpha = 1$ case discussed in the main text. To satisfy these limits we conveniently consider the tagged velocity $v_0 = 3$ and 0, respectively, while drawing the rest of the velocities independently from a Gaussian distribution. In the first figure on the first row, the typical fluctuations of the scaled displacement $y \propto (m - \bar{c}t)/\sqrt{t}$ are Gaussian (shown by the dashed line) while the second figure on the first row shows that the large fluctuations are better described by a large deviation result (shown by the dotted line, where the dashed line plots the Gaussian distribution). In the figure on the second row, we consider the large time limit $t >> t_{\#}(v_0)$, where the PDFs of the appropriately scaled displacement $y \propto t^{-0.56}(m - \bar{c}t)$, at three different times collapse onto a Gaussian distribution shown by dashed line. As discussed in Fig. 4 and shown next in Fig. 6, the exact anomalous scaling is not very clear.

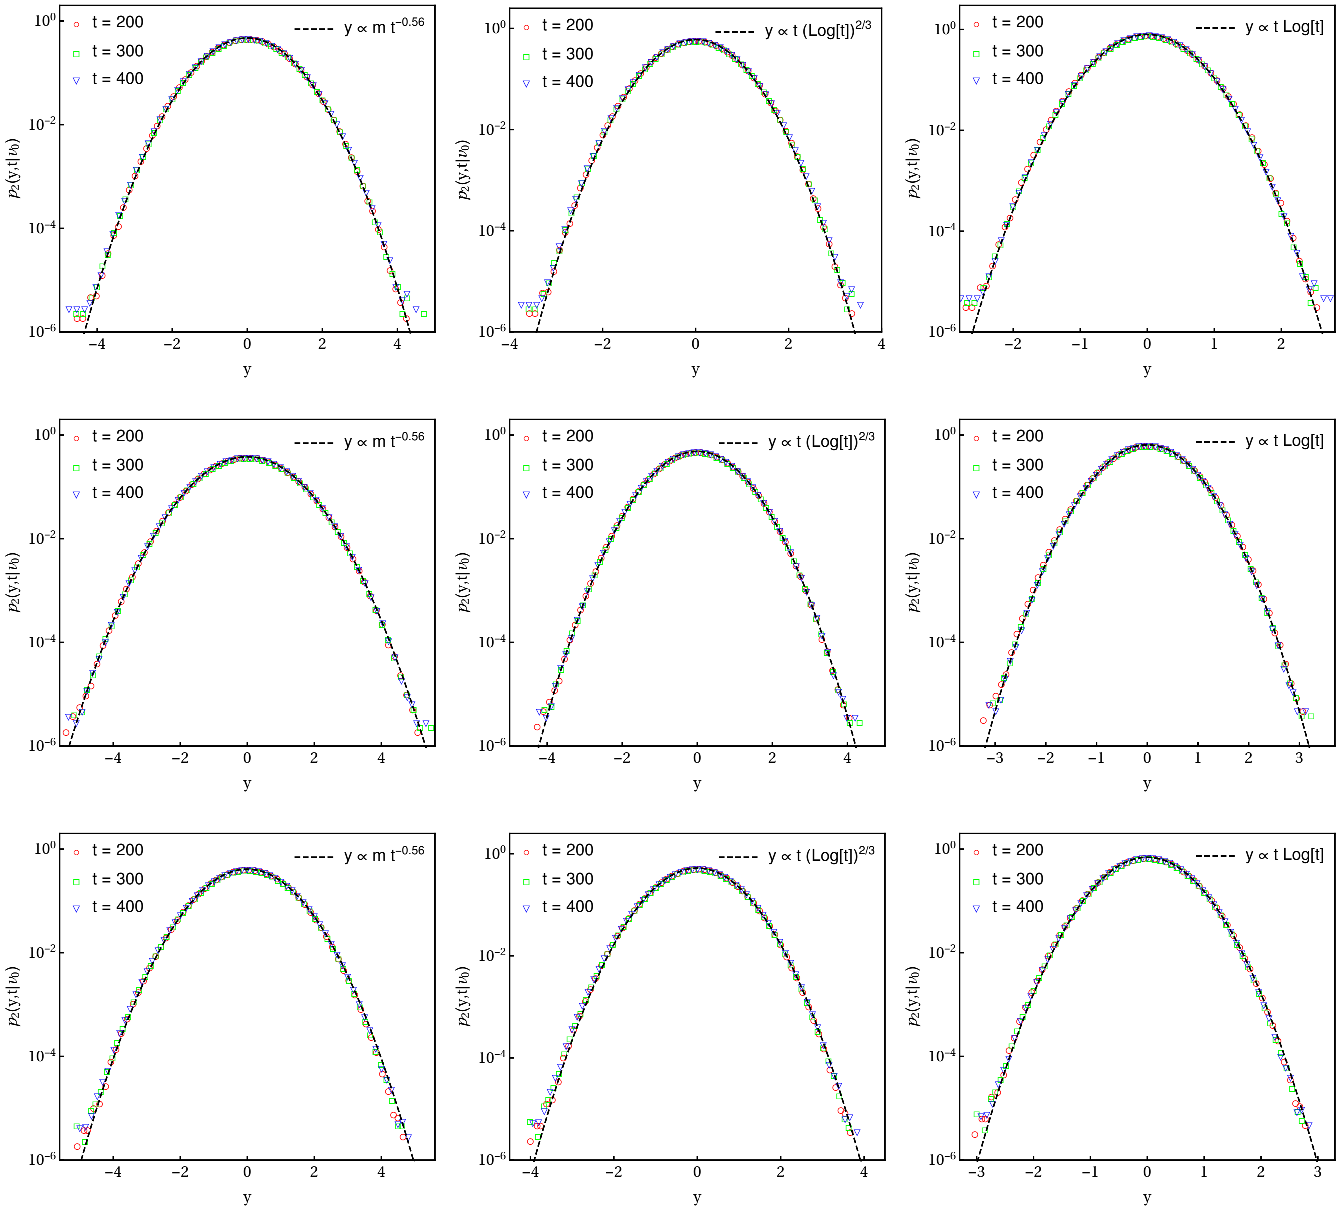


FIG. 6: Conditional PDF of the displacement of a tagged particle with a given velocity $v_0 = \langle v \rangle$, at times $t \gg t_{\#}$, for the $\alpha = 1$ case discussed in the main text. The velocities of the remaining particles are drawn from three different distributions: uniform (first row), Gaussian (second row) and exponential (third row). While the fluctuations of the scaled displacement $y \propto (m - \bar{c}t)/\sigma_t$ is well described by Gaussian (shown by dashed lines), the exact time dependence of the variance is not clear as it matches equally well with $\sigma_t^2 \propto t^{1.12}$ (figures on the first column) as well as $\sigma_t^2 \propto t\,[\mathrm{Log}(t)]^{2\gamma}$ for $\gamma = 1/3$ (figures on the second column) and $\gamma = 1/2$ (figures on the third column).

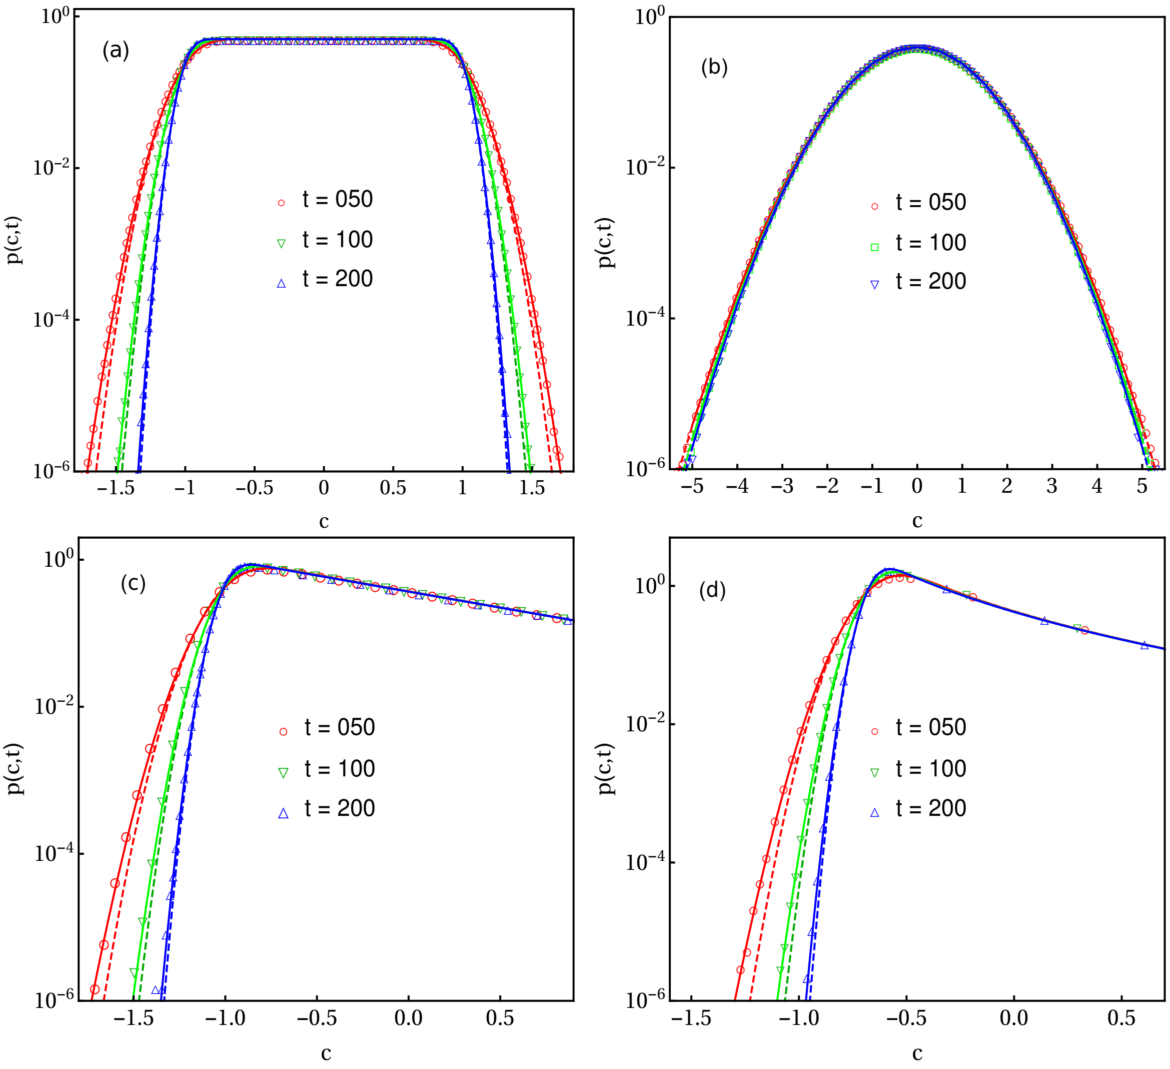


FIG. 7: Probability density function $p(c,t)$ of the scaled net overtakings $c = m(t)/t$ are plotted at three different times, for $\alpha = 1$ case discussed in the main text, with four different choices of the initial velocity distribution, namely, (a) uniform (b) Gaussian (c) exponential and (d) power-law distributions. The discrete points in each plot are the simulation results. They show very good agreement with the results coming from the analysis of the large deviation form of the conditional distribution $p_1(c,t|v_0)$ (as shown by the bold lines). The corresponding results coming from the Gaussian approximation are also plotted (as shown by the dashed lines), for which the agreements at the tails improve as $t$ becomes larger.
